# Supplementary material for: Stochastic Top-$K$ Subset Bandits with Linear Space and Non-Linear Feedback
Source: arXiv:1811.11925 source file (2021-10-11)
Supplement: Supplementary file 1 [file appendix_social_influence1.tex]

\section{Details on Social Influence Maximization}

\subsection{Properties of the Social Influence as a Reward Function }

\label{appendix_social_influence1}
In this appendix we discuss the assumptions of the \NAM \ in the context of Social Influence Maximization.  %In particular, we examine whether the expected diffusion size function $\sigma(\cdot)$ satisfies Assumptions \ref{symmentry_assumption}-\ref{inverse_continuity}. 
% 
%  The diffusion size function $\sigma(\cdot): 2^V \to [0,|V|]$ is a monotonic, non-decreasing, submodular set function \cite{kempe2003maximizing}.  
 The reward $r_{\bf a}(t)$ for an action ${\bf a}$ of choosing seed set $S$ at time $t$ is the count of infected individuals in a cascade run at time $t$ where only nodes in $S$ were initially infected,
%  
%  It is not clear that random influence function for subsets $S \subseteq V$
\[r_{\bf a}(t) = \sum_{v \in V} y_t^{(v)}   \quad \text{ where only } v \in S \text{ were initially influenced}  .\]
It is not clear that the aggregate reward function $r_{\bf a}(t)$ can be decomposed into a function of ``rewards'' for individual nodes like  $f({\bf d}_{{\bf a}_t})$ in \eqref{eq:R_at_t}.  One approach for doing so is using the marginal influence, such as setting the individual reward $X_{i,t}$ of person $i$ at time $t$  as the resulting cascade size if $i$  alone was initially influenced in cascade $t$; then letting the reward $r_{\bf a}(t)$ for the set $S$ be the count of nodes influenced by at least one of the $v \in S$ (e.g., combine the cascades of individual seeds). However, the corresponding reward $r_{\bf a}(t)$ would depend on the overlap of the cascade subgraphs, which depends in part on which seeds $i$ are in $S$ and their relative locations in the network, not just the sizes $\{X_{i,t}\}_{i\in S}$ of the individual cascades.  Thus, defining individual rewards in this way would lead to $r_{\bf a}(t)$ not satisfying the form \eqref{eq:R_at_t} in general, where $f(\cdot)$ should not depend on the specific indices $i \in {\bf a}$.  % For other diffusion models like linear threshold it is even less apparent how you can break apart

\subsection{Computational Complexities of the Methods discussed in Section \ref{social_algorithms}}

\label{appendix_social_influence2}

Table~1 compares the complexities of the different methods discussed in Section \ref{social_algorithms}.  In terms of both time and space complexity, \NAM \ outperforms the other two adaptive methods of influence maximization viz. the UCB algorithm and $\epsilon$-greedy version of credit distribution model.

\begin{table}[h!]
\caption{Computational complexities of methods discussed in Section \ref{social_algorithms}}\label{run_time_table}
\centering
\begin{tabular}{c c c}
\hline \hline
Algorithm & Time-Complexity & Space-Complexity \\
\hline
    CMAB &    $O(K \log K)$ &    $O(N)$\\
    $\epsilon$-CD &  $\Omega(N T^2(1-\epsilon)^2)$ &    $\Omega\left(N T\right)$\\
    UCB &    $O( N^K K \log N )$ &   $O( N^K)$ \\
\hline \\
\end{tabular}
\end{table}
