# Supplementary material for: Stochastic Top-$K$ Subset Bandits with Linear Space and Non-Linear Feedback
Source: arXiv:1811.11925 source file (2021-10-11)
Supplement: Supplementary file 2 [file appendix_social_influence2.tex]

\section{Social Influence Maximization for Florentine Families Network}

\label{appendix_social_influence2}

{\color{blue}
We have also performed real world experiments for the \textit{Florentine families network} \citep{breiger1986cumulated} with 15 nodes with 20 undirected edges. It is a classic network of 15 families in Florence, Italy. Although, the dataset is small, it is relevant to the problem of social influence maximization as families do influence each other's socio-economic behavior.}

We compare the performance of \NAM\ with other methods viz. $\epsilon$-CD algorithm and UCB algorithm for different seed set sizes $K = 2,4,8$ and a time horizon $T=100,000$. Performance of each algorithm was measured using observed reward and expected regret, averaged over 10 runs. For each seed set, the expected influence values, used to determine the optimal set and calculate expected regret, were empirically estimated using 10,000 Monte Carlo simulations. 
{\color{blue}
The observed reward and expected regret for each algorithm, averaged over 10 runs, are shown in Figure \ref{fig:figure_fl_reward} and Figure \ref{fig:figure_fl_regret} respectively, separately for each $K=2,4,8$. \emph{For all values of $K$,} the reward increases and regret decays for \NAM \ at a higher rate than the UCB algorithm (a bandits-specific method). Also, \emph{for all values of $K$,} the reward for \NAM \ approaches to the reward of the optimal set as attained by the much more sophisticated $\epsilon$-CD algorithm (a domain-specific method).  Further, we see that the proposed algorithm outperforms the UCB algorithm.

It is also interesting to note that contrary to the Facebook friends network case, \NAM \ takes much less (almost the same as the $\epsilon$-CD algorithm) time to reach to the optimal set for $K=2,4$ which is because the size of the Florentine families network is much smaller than the Facebook friends network.

\begin{figure}
    \centering
    \begin{subfigure}[b]{0.3\textwidth}
         \centering
        \includegraphics[width=\textwidth]{figures/sim_reward_plot_k_2_fl.eps}
        \caption{$K=2$}
        \label{fig:K_2_fl}
    \end{subfigure}
    \begin{subfigure}[b]{0.3\textwidth}
         \centering
        \includegraphics[width=\textwidth]{figures/sim_reward_plot_k_4_fl.eps}
        \caption{$K=4$}
        \label{fig:K_4_fl}
    \end{subfigure}
    \begin{subfigure}[b]{0.3\textwidth}
         \centering
        \includegraphics[width=\textwidth]{figures/sim_reward_plot_k_8_fl.eps}
        \caption{$K=8$}
        \label{fig:K_8_fl}
    \end{subfigure}
    \caption{Averaged observed reward for different algorithms for different seed set sizes for the \textit{Florentine families network}}
    \label{fig:figure_fl_reward}
\end{figure}

\begin{figure}
    \centering
    \begin{subfigure}[b]{0.3\textwidth}
         \centering
        \includegraphics[width=\textwidth]{figures/sim_regret_plot_k_2_fl.eps}
        \caption{$K=2$}
        \label{fig:K_2_fl}
    \end{subfigure}
    \begin{subfigure}[b]{0.3\textwidth}
         \centering
        \includegraphics[width=\textwidth]{figures/sim_regret_plot_k_4_fl.eps}
        \caption{$K=4$}
        \label{fig:K_4_fl}
    \end{subfigure}
    \begin{subfigure}[b]{0.3\textwidth}
         \centering
        \includegraphics[width=\textwidth]{figures/sim_regret_plot_k_8_fl.eps}
        \caption{$K=8$}
        \label{fig:K_8_fl}
    \end{subfigure}
    \caption{Averaged expected regret for different algorithms for different seed set sizes for the \textit{Florentine families network}}
    \label{fig:figure_fl_regret}
\end{figure}
}

%The difference in performance is most pronounced for smaller $K$ values. This is expected, as with $K=2$, every seed set guarantees $2$ influenced nodes with $13$ nodes left, while for $K=8$ there are only $7$ nodes remaining, so the potential gap between the worst and best sets is smaller. %, and the rate is decreasing as the seed set size increases.
