# Supplementary material for: Stochastic Top-$K$ Subset Bandits with Linear Space and Non-Linear Feedback
Source: arXiv:1811.11925 source file (2021-10-11)
Supplement: Supplementary file 3 [file appendix_social_influence3.tex]

\section{Assumptions for Social Influence Maximization} \label{appendix_social_influence3}

    We note that although several assumptions do not strictly hold for the problem of social influence maximization, related properties do. These are: 
    \begin{enumerate}
        \item Assumption 1 of symmetry: The reward function for the social influence maximization problem is independent of the seed set ordering.     
        
        \item Assumption 4: The social influence maximization objective function is a submodular set function \citep{kempe2003maximizing}, which implies bounds similar to Lipschitz Continuity.        
        
        \item  Assumptions 3 and 5  of strictly increasing and continuous reward function: 
        In the social network, if the influence of a single node increases slightly, such as through increased edge weights, the expected total reward of any seed set containing that node will most often increase, but not drastically so.  
        
        The only situation in which there will be an increase for individual node rewards but no increase in the expected total reward is when only weights on edges between nodes in the seed set are increased.  
        
        Increasing edge weights (and consequently individual node rewards) will never decrease the expected total reward for any seed set.

        % We note that these assumptions do not hold in general. For example, suppose a node is only connected to one other node in the graph and both of the nodes are in the initial seed set. Then increasing the edge weight (infection probability) from the first to the second node will increase the first node's individual influence but will not change the total reward as the second node is always activated. 
        
        % However, these properties hold with high probability as we are selecting initial seed sets uniformly at random, and the probability of selecting all neighbors of a node for that seed set is small.    %$O(K/N)$.  

    \item Stochastic dominance does not hold in general for the problem of social influence maximization.  However, we empirically found that a weaker version of stochastic dominance holds %with some probability for influence maximization.  We describe that property below and provide evidence that this version does hold 
    with non-negligible probability in the network we studied. We now explain this weaker version of stochastic dominance in detail.
    \end{enumerate}

    In Section 6.2, we discussed how influence maximization does not (strictly) satisfy the assumptions of stochastic dominance of individual arms or the reward being a (strictly increasing) function of individual arm rewards.  However, we have empirically found evidence that a related property holds.  We now introduce this related property, a weaker form of stochastic dominance for size $K$ sets.  
    
    Let $a,b \in [N]$ denote two distinct arm indices.  Let $S_{a,b}\in ([N]\backslash \{a,b \})^{K-1}$ denote a random set of $K-1$ distinct  arm indices, uniformly distributed over all ${N-2 \choose K-1 }$ subsets of $[N]\backslash \{a,b \}$ with cardinality $K-1$. 
        
    \textbf{Definition.   Approximate Dominance in Expectation.} Arm $a$ is said to approximately dominate arm $b$ in expectation, with probability $1-\delta$, if
    \begin{align*}
        \text{Prob}\bigg[ &\mathrm{E}_{P_{\bf X}} \big[ f(X_{S_{a,b}(1)}, \dots, X_{S_{a,b}(K-1)}, X_a) \big]\\
        &\geq \mathrm{E}_{P_{\bf X}} \big[ f(X_{S_{a,b}(1)}, \dots, X_{S_{a,b}(K-1)}, X_b) \big] \bigg] = 1-\delta,
    \end{align*}
    where the inner expectations are with respect to the arm distributions and the outer probability is taken with respect to the the uniform measure over possible $S_{a,b}$.
    
    Stochastic dominance, with a symmetric and strictly increasing reward function $f(\cdot)$, implies this dominance in expectation with $\delta=0$.  The converse is not true.  

    %\hl{Empirically, we observe that as $K$ increases, this property holds with lower probability $1-\delta$.  That may in part  explain why the performance gap between UCB and CMAB decreases as $K$ increases.  See Figure XX, specifically the vertical gap between the blue line (XX) and the brown line (XX).}
    
    We empirically assessed the prevalence of this property for the influence maximization problem.     
    
    For each pair of nodes $a$ and $b$ (w.l.o.g. ordered so  $a$ approximately dominates $b$ in expectation), there is a corresponding $1-\delta\geq 0.5$.  We  uniformly sampled from pairs $\{a,b\}$ at random, inducing a probability distribution on the $\delta$ values. 
    
    For each $K=2,4,8$, for 500 different pairs of \{$a,b$\}, we  calculated the above probability over a uniform distribution  over $S_{a,b}$ (based on a 500 random samples from $S_{a,b}$), where the expected influence of any set was calculated as sample average based on 500 diffusions. We observed that the probabilistic stochastic dominance is satisfied with a reasonably high probability.
  
    We  computed the complementary cumulative distribution of $1-\delta$ to indicate what fraction of pairs of nodes $\{a,b\}\subset [N]$ (such that either $a$ or $b$ is in the optimal set for a given $K$) satisfy approximate stochastic dominance with a probability $1-\delta$ of at least a given value.
    
    Figure \ref{fig:stoch_dom_ecdf} displays the empirical complementary cumulative distribution function of $1-\delta$ values for different values of $K$ from \textit{Facebook friends network} \cite{leskovec2012learning}. If stochastic dominance held, then the curves would be flat with a value of $1$.  Thus, higher values indicate stronger dominance.  $K=2$ has the highest values, then $K=4$ and $K=8$ respectively.  Thus, even for $K=8$, for example, about half of all pairs of nodes $\{a,b\}\subset [N]$ satisfy approximate dominance in expectation with a probability of at least $0.9$. %These results suggest that we might expect the proposed algorithm to have a better chance at finding the best set of $K$ nodes when $K$ is smaller, as this approximate form of stochastic dominance holds for more pairs of nodes $\{a,b\}\subset [N]$.  
    
    \begin{figure}[h]
        \centering
        \input{figures/stoch_dom_fb4_new}
        \caption{Complementary CDF of the approximate dominance in expectation probabilities $1-\delta$ for different values of $K$ for the \textit{Facebook friends network}.  The height of each curve indicates what fraction of nodes satisfy this weaker form of dominance.}
        \label{fig:stoch_dom_ecdf}
    \end{figure}
